# Supplementary material for: R-vine Models for Spatial Time Series with an Application to Daily Mean Temperature
Source: arXiv:1403.3500 source file (2014-03-14)
Supplement: Supplementary file 1 [file Appendix.tex]

\begin{appendix}

\section{Outsourced figures}\label{app:fig}

\subsection{Predictions: spatial R-vine model}\label{app:predSV}

\begin{figure}[htb]
	\centering
		\includegraphics[width=1.00\textwidth]{Figures/SVpred01.pdf}
	\caption[Prediction of the mean temperatures for the observation stations $61$, $62$, $72$, $68$, $64$ and $57$ based on the spatial R-vine model.]{Prediction of the mean temperatures for the observation stations $61$, $62$, $72$, $68$, $64$ and $57$ for the period 01/01/2010-12/31/2012 based on the spatial R-vine model. black line: observed values. dark gray line: prediction. light gray area: $95\%$ prediction intervals.}
	\label{fig:SVpred01}
\end{figure}

\begin{figure}[htbp]
	\centering
		\includegraphics[width=1.00\textwidth]{Figures/SVpred02.pdf}
	\caption[Prediction of the mean temperatures for the observation stations $77$, $70$, $56$, $58$, $78$ and $74$ based on the spatial R-vine model.]{Prediction of the mean temperatures for the observation stations $77$, $70$, $56$, $58$, $78$ and $74$ for the period 01/01/2010-12/31/2012 based on the spatial R-vine model. black line: observed values. dark gray line: prediction. light gray area: $95\%$ prediction intervals.}
	\label{fig:SVpred02}
\end{figure}

\begin{figure}[htbp]
	\centering
		\includegraphics[width=1.00\textwidth]{Figures/SVpred03.pdf}
	\caption[Prediction of the mean temperatures for the observation stations $63$, $65$, $60$, $66$, $59$ and $67$ based on the spatial R-vine model.]{Prediction of the mean temperatures for the observation stations $63$, $65$, $60$, $66$, $59$ and $67$ for the period 01/01/2010-12/31/2012 based on the spatial R-vine model. black line: observed values. dark gray line: prediction. light gray area: $95\%$ prediction intervals.}
	\label{fig:SVpred03}
\end{figure}

\begin{figure}[htbp]
	\centering
		\includegraphics[width=1.00\textwidth]{Figures/SVpred04.pdf}
	\caption[Prediction of the mean temperatures for the observation stations $76$, $71$, $55$, $75$, $73$ and $69$ based on the spatial R-vine model.]{Prediction of the mean temperatures for the observation stations $76$, $71$, $55$, $75$, $73$ and $69$ for the period 01/01/2010-12/31/2012 based on the spatial R-vine model. black line: observed values. dark gray line: prediction. light gray area: $95\%$ prediction intervals.}
	\label{fig:SVpred04}
\end{figure}

\begin{figure}[htbp]
	\centering
		\includegraphics[width=1.00\textwidth]{Figures/SVpredres01.pdf}
	\caption[Prediction errors of the predictions for the observation stations $61$, $62$, $72$, $68$, $64$ and $57$ based on the spatial R-vine model.]{Prediction errors of the predictions for the observation stations $61$, $62$, $72$, $68$, $64$ and $57$ for the period 01/01/2010-12/31/2012 based on the spatial R-vine model.}
	\label{fig:SVpredres01}
\end{figure}

\begin{figure}[htbp]
	\centering
		\includegraphics[width=1.00\textwidth]{Figures/SVpredres02.pdf}
	\caption[Prediction errors of the predictions for the observation stations $77$, $70$, $56$, $58$, $78$ and $74$ based on the spatial R-vine model.]{Prediction errors of the predictions for the observation stations $77$, $70$, $56$, $58$, $78$ and $74$ for the period 01/01/2010-12/31/2012 based on the spatial R-vine model.}
	\label{fig:SVpredres02}
\end{figure}

\begin{figure}[htbp]
	\centering
		\includegraphics[width=1.00\textwidth]{Figures/SVpredres03.pdf}
	\caption[Prediction errors of the predictions for the observation stations $63$, $65$, $60$, $66$, $59$ and $67$ based on the spatial R-vine model.]{Prediction errors of the predictions for the observation stations $63$, $65$, $60$, $66$, $59$ and $67$ for the period 01/01/2010-12/31/2012 based on the spatial R-vine model.}
	\label{fig:SVpredres03}
\end{figure}

\begin{figure}[htbp]
	\centering
		\includegraphics[width=1.00\textwidth]{Figures/SVpredres04.pdf}
	\caption[Prediction errors of the predictions for the observation stations $76$, $71$, $55$, $75$, $73$ and $69$ based on the spatial R-vine model.]{Prediction errors of the predictions for the observation stations $76$, $71$, $55$, $75$, $73$ and $69$ for the period 01/01/2010-12/31/2012 based on the spatial R-vine model.}
	\label{fig:SVpredres04}
\end{figure}

%\begin{figure}[htbp]
	%\centering
		%\includegraphics[width=1.00\textwidth]{Figures/SVpredhist01.pdf}
	%\caption[Histograms for $18$ days of the period 01/01/2010-12/31/2012, based on the predictive distribution of the mean temperatures at Albstadt-Badkap (55) (spatial R-vine model).]{Histograms and corresponding kernel density estimates for the last days of the months February, April, June, August, October and December of the years $2010$-$2012$, each calculated from $1000$ simulations from the predictive distribution of the mean temperatures at the observation station Albstadt-Badkap (55) which is based on the spatial R-vine model. Mean and $95\%$ prediction interval are indicated.}
	%\label{fig:SVpredhist01}
%\end{figure}

\begin{figure}[htbp]
	\centering
		\includegraphics[width=1.00\textwidth]{Figures/SVpredbox201.pdf}
	\caption[$95\%$ prediction intervals, point predictions and observed mean temperatures for the first days of each months during the years $2010$-$2012$ for the observation stations $61$, $62$, $72$, $68$, $64$ and $57$, based on the predictive distribution of the respective observation station (spatial R-vine model).]{$95\%$ prediction intervals, point predictions and observed mean temperatures for the first days of each months during the years $2010$-$2012$ for the observation stations $61$, $62$, $72$, $68$, $64$ and $57$, each calculated based on $1000$ simulations from the predictive distribution of the mean temperatures at the respective observation station (spatial R-vine model).}
	\label{fig:SVpredbox01}
\end{figure}

\begin{figure}[htbp]
	\centering
		\includegraphics[width=1.00\textwidth]{Figures/SVpredbox202.pdf}
	\caption[$95\%$ prediction intervals, point predictions and observed mean temperatures for the first days of each months during the years $2010$-$2012$ for the observation stations $77$, $70$, $56$, $58$, $78$ and $74$, based on the predictive distribution of the respective observation station (spatial R-vine model).]{$95\%$ prediction intervals, point predictions and observed mean temperatures for the first days of each months during the years $2010$-$2012$ for the observation stations $77$, $70$, $56$, $58$, $78$ and $74$, each calculated based on $1000$ simulations from the predictive distribution of the mean temperatures at the respective observation station (spatial R-vine model).}
	\label{fig:SVpredbox02}
\end{figure}

\begin{figure}[htbp]
	\centering
		\includegraphics[width=1.00\textwidth]{Figures/SVpredbox203.pdf}
	\caption[$95\%$ prediction intervals, point predictions and observed mean temperatures for the first days of each months during the years $2010$-$2012$ for the observation stations $63$, $65$, $60$, $66$, $59$ and $67$, based on the predictive distribution of the respective observation station (spatial R-vine model).]{$95\%$ prediction intervals, point predictions and observed mean temperatures for the first days of each months during the years $2010$-$2012$ for the observation stations $63$, $65$, $60$, $66$, $59$ and $67$, each calculated based on $1000$ simulations from the predictive distribution of the mean temperatures at the respective observation station (spatial R-vine model).}
	\label{fig:SVpredbox03}
\end{figure}

\begin{figure}[htbp]
	\centering
		\includegraphics[width=1.00\textwidth]{Figures/SVpredbox204.pdf}
	\caption[$95\%$ prediction intervals, point predictions and observed mean temperatures for the first days of each months during the years $2010$-$2012$ for the observation stations $76$, $71$, $55$, $75$, $73$ and $69$, based on the predictive distribution of the respective observation station (spatial R-vine model).]{$95\%$ prediction intervals, point predictions and observed mean temperatures for the first days of each months during the years $2010$-$2012$ for the observation stations $76$, $71$, $55$, $75$, $73$ and $69$, each calculated based on $1000$ simulations from the predictive distribution of the mean temperatures at the respective observation station (spatial R-vine model).}
	\label{fig:SVpredbox04}
\end{figure}

\clearpage

\subsection{Predictions: spatial composite vine model}\label{app:predSCVM}

\begin{figure}[htb]
	\centering
		\includegraphics[width=1.00\textwidth]{Figures/SCVMpred01.pdf}
	\caption[Prediction of the mean temperatures for the observation stations $61$, $62$, $72$, $68$, $64$ and $57$ based on the spatial composite vine model.]{Prediction of the mean temperatures for the observation stations $61$, $62$, $72$, $68$, $64$ and $57$ for the period 01/01/2010-12/31/2012 based on the spatial composite vine model. black line: observed values. dark gray line: prediction. light gray area: $95\%$ prediction intervals.}
	\label{fig:SCVMpred01}
\end{figure}

\begin{figure}[htbp]
	\centering
		\includegraphics[width=1.00\textwidth]{Figures/SCVMpred02.pdf}
	\caption[Prediction of the mean temperatures for the observation stations $77$, $70$, $56$, $58$, $78$ and $74$ based on the spatial composite vine model.]{Prediction of the mean temperatures for the observation stations $77$, $70$, $56$, $58$, $78$ and $74$ for the period 01/01/2010-12/31/2012 based on the spatial composite vine model. black line: observed values. dark gray line: prediction. light gray area: $95\%$ prediction intervals.}
	\label{fig:SCVMpred02}
\end{figure}

\begin{figure}[htbp]
	\centering
		\includegraphics[width=1.00\textwidth]{Figures/SCVMpred03.pdf}
	\caption[Prediction of the mean temperatures for the observation stations $63$, $65$, $60$, $66$, $59$ and $67$ based on the spatial composite vine model.]{Prediction of the mean temperatures for the observation stations $63$, $65$, $60$, $66$, $59$ and $67$ for the period 01/01/2010-12/31/2012 based on the spatial composite vine model. black line: observed values. dark gray line: prediction. light gray area: $95\%$ prediction intervals.}
	\label{fig:SCVMpred03}
\end{figure}

\begin{figure}[htbp]
	\centering
		\includegraphics[width=1.00\textwidth]{Figures/SCVMpred04.pdf}
	\caption[Prediction of the mean temperatures for the observation stations $76$, $71$, $55$, $75$, $73$ and $69$ based on the spatial composite vine model.]{Prediction of the mean temperatures for the observation stations $76$, $71$, $55$, $75$, $73$ and $69$ for the period 01/01/2010-12/31/2012 based on the spatial composite vine model. black line: observed values. dark gray line: prediction. light gray area: $95\%$ prediction intervals.}
	\label{fig:SCVMpred04}
\end{figure}

\begin{figure}[htbp]
	\centering
		\includegraphics[width=1.00\textwidth]{Figures/SCVMpredres01.pdf}
	\caption[Prediction errors of the predictions for the observation stations $61$, $62$, $72$, $68$, $64$ and $57$ based on the spatial composite vine model.]{Prediction errors of the predictions for the observation stations $61$, $62$, $72$, $68$, $64$ and $57$ for the period 01/01/2010-12/31/2012 based on the spatial composite vine model.}
	\label{fig:SCVMpredres01}
\end{figure}

\begin{figure}[htbp]
	\centering
		\includegraphics[width=1.00\textwidth]{Figures/SCVMpredres02.pdf}
	\caption[Prediction errors of the predictions for the observation stations $77$, $70$, $56$, $58$, $78$ and $74$ based on the spatial composite vine model.]{Prediction errors of the predictions for the observation stations $77$, $70$, $56$, $58$, $78$ and $74$ for the period 01/01/2010-12/31/2012 based on the spatial composite vine model.}
	\label{fig:SCVMpredres02}
\end{figure}

\begin{figure}[htbp]
	\centering
		\includegraphics[width=1.00\textwidth]{Figures/SCVMpredres03.pdf}
	\caption[Prediction errors of the predictions for the observation stations $63$, $65$, $60$, $66$, $59$ and $67$ based on the spatial composite vine model.]{Prediction errors of the predictions for the observation stations $63$, $65$, $60$, $66$, $59$ and $67$ for the period 01/01/2010-12/31/2012 based on the spatial composite vine model.}
	\label{fig:SCVMpredres03}
\end{figure}

\begin{figure}[htbp]
	\centering
		\includegraphics[width=1.00\textwidth]{Figures/SCVMpredres04.pdf}
	\caption[Prediction errors of the predictions for the observation stations $76$, $71$, $55$, $75$, $73$ and $69$ based on the spatial composite vine model.]{Prediction errors of the predictions for the observation stations $76$, $71$, $55$, $75$, $73$ and $69$ for the period 01/01/2010-12/31/2012 based on the spatial composite vine model.}
	\label{fig:SCVMpredres04}
\end{figure}

%\begin{figure}[htbp]
	%\centering
		%\includegraphics[width=1.00\textwidth]{Figures/SCVMpredhist01.pdf}
	%\caption[Histograms for $18$ days of the period 01/01/2010-12/31/2012, based on the predictive distribution of the mean temperatures at Albstadt-Badkap (55) (spatial composite vine model).]{Histograms and corresponding kernel density estimates for the last days of the months February, April, June, August, October and December of the years $2010$-$2012$, each calculated from $1000$ simulations from the predictive distribution of the mean temperatures at the observation station Albstadt-Badkap (55) which is based on the spatial composite vine model. Mean and $95\%$ prediction interval are indicated.}
	%\label{fig:SCVMpredhist01}
%\end{figure}

\begin{figure}[htbp]
	\centering
		\includegraphics[width=1.00\textwidth]{Figures/SCVMpredbox201.pdf}
	\caption[$95\%$ prediction intervals, point predictions and observed mean temperatures for the first days of each months during the years $2010$-$2012$ for the observation stations $61$, $62$, $72$, $68$, $64$ and $57$, based on the predictive distribution of the respective observation station (spatial composite vine model).]{$95\%$ prediction intervals, point predictions and observed mean temperatures for the first days of each months during the years $2010$-$2012$ for the observation stations $61$, $62$, $72$, $68$, $64$ and $57$, each calculated based on $1000$ simulations from the predictive distribution of the mean temperatures at the respective observation station (spatial composite vine model).}
	\label{fig:SCVMpredbox01}
\end{figure}

\begin{figure}[htbp]
	\centering
		\includegraphics[width=1.00\textwidth]{Figures/SCVMpredbox202.pdf}
	\caption[$95\%$ prediction intervals, point predictions and observed mean temperatures for the first days of each months during the years $2010$-$2012$ for the observation stations $77$, $70$, $56$, $58$, $78$ and $74$, based on the predictive distribution of the respective observation station (spatial composite vine model).]{$95\%$ prediction intervals, point predictions and observed mean temperatures for the first days of each months during the years $2010$-$2012$ for the observation stations $77$, $70$, $56$, $58$, $78$ and $74$, each calculated based on $1000$ simulations from the predictive distribution of the mean temperatures at the respective observation station (spatial composite vine model).}
	\label{fig:SCVMpredbox02}
\end{figure}

\begin{figure}[htbp]
	\centering
		\includegraphics[width=1.00\textwidth]{Figures/SCVMpredbox203.pdf}
	\caption[$95\%$ prediction intervals, point predictions and observed mean temperatures for the first days of each months during the years $2010$-$2012$ for the observation stations $63$, $65$, $60$, $66$, $59$ and $67$, based on the predictive distribution of the respective observation station (spatial composite vine model).]{$95\%$ prediction intervals, point predictions and observed mean temperatures for the first days of each months during the years $2010$-$2012$ for the observation stations $63$, $65$, $60$, $66$, $59$ and $67$, each calculated based on $1000$ simulations from the predictive distribution of the mean temperatures at the respective observation station (spatial composite vine model).}
	\label{fig:SCVMpredbox03}
\end{figure}

\begin{figure}[htbp]
	\centering
		\includegraphics[width=1.00\textwidth]{Figures/SCVMpredbox204.pdf}
	\caption[$95\%$ prediction intervals, point predictions and observed mean temperatures for the first days of each months during the years $2010$-$2012$ for the observation stations $76$, $71$, $55$, $75$, $73$ and $69$, based on the predictive distribution of the respective observation station (spatial composite vine model).]{$95\%$ prediction intervals, point predictions and observed mean temperatures for the first days of each months during the years $2010$-$2012$ for the observation stations $76$, $71$, $55$, $75$, $73$ and $69$, each calculated based on $1000$ simulations from the predictive distribution of the mean temperatures at the respective observation station (spatial composite vine model).}
	\label{fig:SCVMpredbox04}
\end{figure}

\clearpage

\subsection{Predictions: spatial Gaussian model}\label{app:predSG}

\begin{figure}[htb]
	\centering
		\includegraphics[width=1.00\textwidth]{Figures/STpred01.pdf}
	\caption[Prediction of the mean temperatures for the observation stations $61$, $62$, $72$, $68$, $64$ and $57$ based on the spatial Gaussian model.]{Prediction of the mean temperatures for the observation stations $61$, $62$, $72$, $68$, $64$ and $57$ for the period 01/01/2010-12/31/2012 based on the spatial Gaussian model. black line: observed values. dark gray line: prediction. light gray area: $95\%$ prediction intervals.}
	\label{fig:STpred01}
\end{figure}

\begin{figure}[htbp]
	\centering
		\includegraphics[width=1.00\textwidth]{Figures/STpred02.pdf}
	\caption[Prediction of the mean temperatures for the observation stations $77$, $70$, $56$, $58$, $78$ and $74$ based on the spatial Gaussian model.]{Prediction of the mean temperatures for the observation stations $77$, $70$, $56$, $58$, $78$ and $74$ for the period 01/01/2010-12/31/2012 based on the spatial Gaussian model. black line: observed values. dark gray line: prediction. light gray area: $95\%$ prediction intervals.}
	\label{fig:STpred02}
\end{figure}

\begin{figure}[htbp]
	\centering
		\includegraphics[width=1.00\textwidth]{Figures/STpred03.pdf}
	\caption[Prediction of the mean temperatures for the observation stations $63$, $65$, $60$, $66$, $59$ and $67$ based on the spatial Gaussian model.]{Prediction of the mean temperatures for the observation stations $63$, $65$, $60$, $66$, $59$ and $67$ for the period 01/01/2010-12/31/2012 based on the spatial Gaussian model. black line: observed values. dark gray line: prediction. light gray area: $95\%$ prediction intervals.}
	\label{fig:STpred03}
\end{figure}

\begin{figure}[htbp]
	\centering
		\includegraphics[width=1.00\textwidth]{Figures/STpred04.pdf}
	\caption[Prediction of the mean temperatures for the observation stations $76$, $71$, $55$, $75$, $73$ and $69$ based on the spatial Gaussian model.]{Prediction of the mean temperatures for the observation stations $76$, $71$, $55$, $75$, $73$ and $69$ for the period 01/01/2010-12/31/2012 based on the spatial Gaussian model. black line: observed values. dark gray line: prediction. light gray area: $95\%$ prediction intervals.}
	\label{fig:STpred04}
\end{figure}

\begin{figure}[htbp]
	\centering
		\includegraphics[width=1.00\textwidth]{Figures/STpredres01.pdf}
	\caption[Prediction errors of the predictions for the observation stations $61$, $62$, $72$, $68$, $64$ and $57$ based on the spatial Gaussian model.]{Prediction errors of the predictions for the observation stations $61$, $62$, $72$, $68$, $64$ and $57$ for the period 01/01/2010-12/31/2012 based on the spatial Gaussian model.}
	\label{fig:STpredres01}
\end{figure}

\begin{figure}[htbp]
	\centering
		\includegraphics[width=1.00\textwidth]{Figures/STpredres02.pdf}
	\caption[Prediction errors of the predictions for the observation stations $77$, $70$, $56$, $58$, $78$ and $74$ based on the spatial Gaussian model.]{Prediction errors of the predictions for the observation stations $77$, $70$, $56$, $58$, $78$ and $74$ for the period 01/01/2010-12/31/2012 based on the spatial Gaussian model.}
	\label{fig:STpredres02}
\end{figure}

\begin{figure}[htbp]
	\centering
		\includegraphics[width=1.00\textwidth]{Figures/STpredres03.pdf}
	\caption[Prediction errors of the predictions for the observation stations $63$, $65$, $60$, $66$, $59$ and $67$ based on the spatial Gaussian model.]{Prediction errors of the predictions for the observation stations $63$, $65$, $60$, $66$, $59$ and $67$ for the period 01/01/2010-12/31/2012 based on the spatial Gaussian model.}
	\label{fig:STpredres03}
\end{figure}

\begin{figure}[htbp]
	\centering
		\includegraphics[width=1.00\textwidth]{Figures/STpredres04.pdf}
	\caption[Prediction errors of the predictions for the observation stations $76$, $71$, $55$, $75$, $73$ and $69$ based on the spatial Gaussian model.]{Prediction errors of the predictions for the observation stations $76$, $71$, $55$, $75$, $73$ and $69$ for the period 01/01/2010-12/31/2012 based on the spatial Gaussian model.}
	\label{fig:STpredres04}
\end{figure}

%\begin{figure}[htbp]
	%\centering
		%\includegraphics[width=1.00\textwidth]{Figures/STpredhist01.pdf}
	%\caption[Histograms for $18$ days of the period 01/01/2010-12/31/2012, based on the predictive distribution of the mean temperatures at Albstadt-Badkap (55) (spatial Gaussian model).]{Histograms and corresponding kernel density estimates for the last days of the months February, April, June, August, October and December of the years $2010$-$2012$, each calculated from $1000$ simulations from the predictive distribution of the mean temperatures at the observation station Albstadt-Badkap (55) which is based on the spatial Gaussian model. Mean and $95\%$ prediction interval are indicated.}
	%\label{fig:STpredhist01}
%\end{figure}

\begin{figure}[htbp]
	\centering
		\includegraphics[width=1.00\textwidth]{Figures/STpredbox201.pdf}
	\caption[$95\%$ prediction intervals, point predictions and observed mean temperatures for the first days of each months during the years $2010$-$2012$ for the observation stations $61$, $62$, $72$, $68$, $64$ and $57$, based on the predictive distribution of the respective observation station (spatial Gaussian model).]{$95\%$ prediction intervals, point predictions and observed mean temperatures for the first days of each months during the years $2010$-$2012$ for the observation stations $61$, $62$, $72$, $68$, $64$ and $57$, each calculated based on $1000$ simulations from the predictive distribution of the mean temperatures at the respective observation station (spatial Gaussian model).}
	\label{fig:STpredbox01}
\end{figure}

\begin{figure}[htbp]
	\centering
		\includegraphics[width=1.00\textwidth]{Figures/STpredbox202.pdf}
	\caption[$95\%$ prediction intervals, point predictions and observed mean temperatures for the first days of each months during the years $2010$-$2012$ for the observation stations $77$, $70$, $56$, $58$, $78$ and $74$, based on the predictive distribution of the respective observation station (spatial Gaussian model).]{$95\%$ prediction intervals, point predictions and observed mean temperatures for the first days of each months during the years $2010$-$2012$ for the observation stations $77$, $70$, $56$, $58$, $78$ and $74$, each calculated based on $1000$ simulations from the predictive distribution of the mean temperatures at the respective observation station (spatial Gaussian model).}
	\label{fig:STpredbox02}
\end{figure}

\begin{figure}[htbp]
	\centering
		\includegraphics[width=1.00\textwidth]{Figures/STpredbox203.pdf}
	\caption[$95\%$ prediction intervals, point predictions and observed mean temperatures for the first days of each months during the years $2010$-$2012$ for the observation stations $63$, $65$, $60$, $66$, $59$ and $67$, based on the predictive distribution of the respective observation station (spatial Gaussian model).]{$95\%$ prediction intervals, point predictions and observed mean temperatures for the first days of each months during the years $2010$-$2012$ for the observation stations $63$, $65$, $60$, $66$, $59$ and $67$, each calculated based on $1000$ simulations from the predictive distribution of the mean temperatures at the respective observation station (spatial Gaussian model).}
	\label{fig:STpredbox03}
\end{figure}

\begin{figure}[htbp]
	\centering
		\includegraphics[width=1.00\textwidth]{Figures/STpredbox204.pdf}
	\caption[$95\%$ prediction intervals, point predictions and observed mean temperatures for the first days of each months during the years $2010$-$2012$ for the observation stations $76$, $71$, $55$, $75$, $73$ and $69$, based on the predictive distribution of the respective observation station (spatial Gaussian model).]{$95\%$ prediction intervals, point predictions and observed mean temperatures for the first days of each months during the years $2010$-$2012$ for the observation stations $76$, $71$, $55$, $75$, $73$ and $69$, each calculated based on $1000$ simulations from the predictive distribution of the mean temperatures at the respective observation station (spatial Gaussian model).}
	\label{fig:STpredbox04}
\end{figure}

\clearpage

\subsection{Predictions for the 20th of January 2010}\label{app:pred}

\begin{landscape}
\begin{figure}[htbp]
  \centering
  \begin{subfigure}[b]{0.7\textwidth}
    \centering
    \includegraphics[width=\textwidth]{Figures/SCVMpredgrid201.pdf}
    %\caption{SCVMpredgrid201.}
    \label{fig:SCVMpredgrid201}
  \end{subfigure}%
    %add desired spacing between images, e. g. ~, \quad, \qquad etc.
    %(or a blank line to force the subfigure onto a new line)
  \begin{subfigure}[b]{0.7\textwidth}
    \centering
    \includegraphics[width=\textwidth]{Figures/STpredgrid201.pdf}
    %\caption{STpredgrid201.}
    \label{fig:STpredgrid201}
  \end{subfigure}%
        \caption[Level plots comparing predictions (spatial composite vine model vs. spatial Gaussian model) on a $80\times120$ grid on the $20$th of January $2010$.]{Level plots comparing predictions based on the spatial composite vine model and the spatial Gaussian model on a $80\times120$ grid covering Germany on the $20$th of January $2010$. Whereas the circles represent the mean temperatures at the $54$ observation stations of the training data set, the squares depict the mean temperatures at the $24$ stations of the validation data set.}
				\label{fig:predgrid201}
\end{figure}
\end{landscape}

\begin{landscape}
\begin{figure}[htbp]
  \centering
  \begin{subfigure}[b]{0.7\textwidth}
    \centering
    \includegraphics[width=\textwidth]{Figures/Diffpredgrid201.pdf}
    %\caption{Diffpredgrid201.}
    \label{fig:Diffpredgrid201}
  \end{subfigure}%
    %add desired spacing between images, e. g. ~, \quad, \qquad etc.
    %(or a blank line to force the subfigure onto a new line)
  \begin{subfigure}[b]{0.7\textwidth}
    \centering
    \includegraphics[width=\textwidth]{Figures/Diffpredgrid202.pdf}
    %\caption{Diffpredgrid201.}
    \label{fig:Diffpredgrid202}
  \end{subfigure}%
        \caption[Level plots of (the absolute value of) the difference between the predictions based on the spatial composite vine model and the spatial Gaussian model on a $80\times120$ grid covering Germany on the $20$th of January $2010$.]{Level plots of (the absolute value of) the difference between the predictions based on the spatial composite vine model and the spatial Gaussian model on a $80\times120$ grid covering Germany on the $20$th of January $2010$.}
				\label{fig:Diffpredgrid2}
\end{figure}
\end{landscape}

\begin{landscape}
\begin{figure}[htbp]
  \centering
  \begin{subfigure}[b]{0.7\textwidth}
    \centering
    \includegraphics[width=\textwidth]{Figures/SCVMpredgrid202.pdf}
    %\caption{SCVMpredgrid202.}
    \label{fig:SCVMpredgrid202}
  \end{subfigure}%
    %add desired spacing between images, e. g. ~, \quad, \qquad etc.
    %(or a blank line to force the subfigure onto a new line)
  \begin{subfigure}[b]{0.7\textwidth}
    \centering
    \includegraphics[width=\textwidth]{Figures/STpredgrid202.pdf}
    %\caption{STpredgrid202.}
    \label{fig:STpredgrid202}
  \end{subfigure}%
        \caption[Level plots comparing the $5\%$ quantiles of predictions (spatial composite vine model vs. spatial Gaussian model) on a $80\times120$ grid on the $20$th of January $2010$.]{Level plots comparing the $5\%$ quantiles of predictions based on the spatial composite vine model and the spatial Gaussian model on a $80\times120$ grid covering Germany on the $20$th of January $2010$. Whereas the circles represent the mean temperatures at the $54$ observation stations of the training data set, the squares depict the mean temperatures at the $24$ stations of the validation data set.}
				\label{fig:predgrid202}
\end{figure}
\end{landscape}

\begin{landscape}
\begin{figure}[htbp]
  \centering
  \begin{subfigure}[b]{0.7\textwidth}
    \centering
    \includegraphics[width=\textwidth]{Figures/SCVMpredgrid203.pdf}
    %\caption{SCVMpredgrid203.}
    \label{fig:SCVMpredgrid203}
  \end{subfigure}%
    %add desired spacing between images, e. g. ~, \quad, \qquad etc.
    %(or a blank line to force the subfigure onto a new line)
  \begin{subfigure}[b]{0.7\textwidth}
    \centering
    \includegraphics[width=\textwidth]{Figures/STpredgrid203.pdf}
    %\caption{STpredgrid203.}
    \label{fig:STpredgrid203}
  \end{subfigure}%
        \caption[Level plots comparing the $95\%$ quantiles of predictions (spatial composite vine model vs. spatial Gaussian model) on a $80\times120$ grid on the $20$th of January $2010$.]{Level plots comparing the $95\%$ quantiles of predictions based on the spatial composite vine model and the spatial Gaussian model on a $80\times120$ grid covering Germany on the $20$th of January $2010$. Whereas the circles represent the mean temperatures at the $54$ observation stations of the training data set, the squares depict the mean temperatures at the $24$ stations of the validation data set.}
				\label{fig:predgrid203}
\end{figure}
\end{landscape}

\begin{landscape}
\begin{figure}[htbp]
  \centering
  \begin{subfigure}[b]{0.7\textwidth}
    \centering
    \includegraphics[width=\textwidth]{Figures/SCVMLengthpredinterval2.pdf}
    %\caption{SCVMLengthpredinterval2.}
    \label{fig:SCVMLengthpredinterval2}
  \end{subfigure}%
    %add desired spacing between images, e. g. ~, \quad, \qquad etc.
    %(or a blank line to force the subfigure onto a new line)
  \begin{subfigure}[b]{0.7\textwidth}
    \centering
    \includegraphics[width=\textwidth]{Figures/STLengthpredinterval2.pdf}
    %\caption{STLengthpredinterval2.}
    \label{fig:StLengthpredinterval2}
  \end{subfigure}%
        \caption[Level plots comparing the lengths of the $90\%$ prediction intervals (spatial composite vine model vs. spatial Gaussian model) on a $80\times120$ grid on the $20$th of January $2010$.]{Level plots comparing the lengths of the $90\%$ prediction intervals based on the spatial composite vine model and the spatial Gaussian model on a $80\times120$ grid covering Germany on the $20$th of January $2010$. The circles represent the $54$ observation stations of the training data set, the squares mark the locations of the $24$ stations of the validation data set.}
				\label{fig:Lengthpredinterval2}
\end{figure}
\end{landscape}

\end{appendix}

\cleardoublepage
